# Supplementary material for: How Two-Layer Neural Networks Learn, One (Giant) Step at a Time
Source: arXiv:2305.18270 source file (2025-06-03)
Supplement: Supplementary file 1 [file garbage.tex]

\subsection*{Overview of relevant figures}
\paragraph{Main}
\begin{itemize}[noitemsep,leftmargin=1em]
    \item Fig.~\ref{fig:stairway} - Toy sketch that highlights the different learning regime as a function of the batch size $n$. \textcolor{orange}{LP: Working on making this non-toyish.}
    \item Fig.~\ref{fig:no_spec} - Referring to "Thm 1" - In the $n = O(d)$ regime there is no specialization after finite number of steps ($T = 16$). Moreover, we can predict the neuron orientation in the subspace (red line in the plot). 
    \item Fig.~\ref{fig:d2_d3_regimes} - Referring to Thm 2\&Thm3 - Specialization (or lack thereof) after one big step in the $n = \mathcal{O}(d^l)$ regime - Comparison of a) linear + square; b) 2nd hermite; c) 3rd hermite; 4) 4th hermite. 
    
    % \textcolor{orange}{LP: In Fig.~\ref{fig:d2_regime_mod}\& Fig.~\ref{fig:d3_regime} you can find the disentagled version of this figure if we think is too dense.}
    % \item Fig.~\ref{fig:d2_regime_mod} - Referring to "Thm 2" - Specialization (or lack thereof) after one big step in the $n = \mathcal{O}(d^2)$ regime - Comparison of a) linear + square; b) 2nd hermite; c) pure square function; d) 3rd hermite. The non-linearities $(a,c)$ will not satisfy the hypothesis of the the theorem having non-zero first hermite coefficients $<2$. Function $c)$ will work since its first Hermite different from zero is the second. Function $d)$ won't work since the first non-zero Hermite is the third.  
    % \item Fig.~\ref{fig:d3_regime} Referring to "Thm"3: - Specialization (or lack thereof) after one big step in the $n = \mathcal{O}(d^3)$ - We compare a) linear + square; b) hermite3; c) hermite4. Similar to the quadratic regime, only the hermite3 will respect the hypothesis of Theorem 3. 
\end{itemize}

\paragraph{Appendix}
\begin{itemize}[noitemsep,leftmargin=1em]
    \item \textcolor{orange}{LP: TO-upload} Referring to "Thm 1" - Show logarithmic dependence to specialization $T_{spec} \sim \log{d}$. 
    \item \textcolor{orange}{LP: TO-upload - Goes in appendix?} - Referring to Thm 2 - By updating the second layer we can approximately "remove the first Hermite coefficient". 
    \item \textcolor{orange}{LP: TO-upload, goes in appendix.} Referring to Thms 2\&3, argue numerically that phenomenology does not change for different regime of $p$.
\end{itemize}
