# Supplementary material for: How Two-Layer Neural Networks Learn, One (Giant) Step at a Time
Source: arXiv:2305.18270 source file (2025-06-03)
Supplement: Supplementary file 2 [file bigpicture.tex]

\section{Conceptual Overview and illustrative Examples}\label{app:overview}
